# Supplementary material for: VisualVoice: Audio-Visual Speech Separation with Cross-Modal Consistency
Source: arXiv:2101.03149 source file (2021-04-06)
Supplement: Supplementary file 1 [file 07_supplementary.tex]

%\clearpage
\appendix 

\noindent The supplementary materials for~\cite{gao2021VisualVoice} consist of:
\begin{enumerate}
    \item[A.] Broader impact.
	\item[B.] Supplementary video.
	\item[C.] General single-speaker model VS.~dedicated two-speaker model.
	\item[D.] Separation results for seen-heard speakers VS. unseen-unheard speakers.
	\item[E.] Ablation study on the loss terms.
	\item[F.] Best/worst performing pairs.
	\item[G.] Network and implementation details.
	\item[H.] Dataset details.
\end{enumerate}

%===========================================================
\section{Broader Impact}

We are conscious of possible undesirable effects that can arise when working with data-driven approaches to human understanding in images and video. Specifically, a method's training data will guide the extent to which the model can generalize well and fairly to arbitrary inputs. To mitigate risks in this regard, we have taken several steps. First, we learn the cross-modal face-voice embeddings from the VoxCeleb2 dataset, which to our knowledge is the largest relevant available dataset with over 6,000 speakers spanning a range of different ethnicities, accents, professions, and ages. Second, we examine the speech separation results separately for a seen-heard test set and an unseen-unheard test set from VoxCeleb2. The results show our method achieves similar performance for seen-heard and unseen-unheard speakers. This shows that our model generalizes well to unseen-unheard speakers in VoxCeleb2 and is not limited to handling seen-heard speakers in the training data. 

Finally, the output of our model consists of voices separated from the the original test video---in terms of masking the input spectrogram---as opposed to being generated or machine synthesized. This is important because it means our model is not free to hallucinate arbitrary voice sounds for the input speakers, e.g., the model cannot artificially conjure sounds or words often associated with training faces that happen to look like the input speaker unless they are consistent with the input sounds. Indeed, as shown in results in the main paper, lip motion continues to play a key role during speech separation, isolating words based on their visual agreement with what was physically spoken. The learned cross-modal face-voice embeddings complement lip motion cues to further enhance the separation results, particularly when lip motion is harder to read or the two input faces are very different in appearance.

To further explore the model's performance as a function of a person's race, gender, ethnicity, or other identity data, it would be interesting to sort results by the relative impact of our model along each dimension independently. However, existing meta-data does not permit this study (VoxCeleb2 only provides identity and gender labels). We hope to analyze the per-category performance of our models for these cross-modal speaker attributes when datasets as such meta-data and/or new dataset efforts become available. 

%===========================================================
\section{Supplementary Video}
In the supplementary video\footnote{\url{http://vision.cs.utexas.edu/projects/VisualVoice/}}, we show example separation results. We first show audio-visual speech separation and enhancement results on \textbf{real-world test videos} of multiple speakers in various challenging scenarios including presidential debates, zoom calls, interviews, and noisy restaurants. Next, we show some qualitative results on synthetic mixtures from the VoxCeleb2 dataset and compare with the AV-Conv~\cite{afouras2018conversation} baseline and our static face based model. Finally, we show some failure cases of our model.

%===========================================================
\section{General Single-Speaker Model VS. Dedicated Two-Speaker Model} 

As mentioned in Sec.~3.2 in the main paper, we can either build an audio-visual feature map for each speaker in the mixture to separate their respective voices or build a model tailored to two-speaker speech separation. For the former case, the model can be generally applicable in testing scenarios where the number of speakers is unknown, while the latter only applies to two-speaker speech separation but can benefit from the contextual visual information of the other speaker in the mixture. For audio-visual speech separation on VoxCeleb2, the model tailored to two-speaker speech separation achieves SDR of 10.2, while the general single-speaker model achieves SDR of 9.88. Most of our experiments are on two-speaker speech mixtures due to its wide applications in real-world. Note that a model tailored to more than two speakers can be similarly built by concatenating the visual features of all the speakers in the mixture.

%===========================================================
\section{Separation Results for Seen-Heard Speakers VS. Unseen-Unheard Speakers} 

Table~\ref{Table:av-speech-separation-supp} shows the speech separation results separately for the seen-heard test set and the unseen-unheard test set on the VoxCeleb2 dataset. We can see that the methods purely based on lip motion tend to have similar performance for seen-heard and unseen-unheard speakers. For models that reply on facial appearance, the separation performance is slightly better on the seen-heard test set because the learned cross-model face-voice embeddings are more reliable for seen-heard speakers. Our method leverages both the lip motion and the cross-modal facial attributes, generalizing well to unseen-unheard speakers. 

To further verify that it is beneficial to disentangle lip motion and cross-modal facial attributes, we show a baseline called Face-Track, which directly processes the full face track to extract visual features similar to prior work~\cite{ephrat2018looking}. The gain of our method demonstrates that it is helpful to focus specifically on the lip regions (mouth ROIs) when analyzing the lip movements for separation, and the cross-modal face-voice embeddings learned through our multi-task learning framework can better exploit the complementary facial appearance cues to enhance separation.

\begin{table*}[ht]
\begin{tabular}{c?{0.5mm}ccccc?{0.5mm}ccccc}
\multirow{2}{*}{} & \multicolumn{5}{c?{0.5mm}}{Seen-Heard} & \multicolumn{5}{c}{Unseen Unheard} \\ \cline{2-11} 
                  & SDR    & SIR    & SAR   & PESQ & STOI & SDR    & SIR    & SAR  & PESQ & STOI \\ \specialrule{.12em}{.1em}{.1em}
Audio-Only~\cite{yu2017permutation}   &    8.00     &     13.9       & 10.1    &  2.63  & 0.82 & 7.70     &     13.6       &  9.85    &  2.59  & 0.82\\ 
AV-Conv~\cite{afouras2018conversation}        &   8.94      &   14.8    &   11.2     &   2.73  & 0.84 & 8.89    &  14.8    &  11.1  & 2.72 & 0.84 \\ 
Face-Track       &   9.28      &   15.8    &   11.2     &   2.76   & 0.85 &  9.20      &   15.6    &   11.0     &   2.75   & 0.84  \\ 
Ours (static face)        &   7.37      &  12.2    &   10.7     &  2.54  & 0.80 & 7.06     &  11.8    &   10.6     &  2.49  & 0.80\\ 
Ours (lip motion)   &   9.96  &   16.9      &  11.2    &   2.81     &  0.86   & 9.94 & 17.0  &  11.1   &  2.80  & 0.87  \\ 
Ours        &  \textbf{10.3}      &    \textbf{17.2}    &     \textbf{11.4}   &     \textbf{2.83}     & \textbf{0.87} & \textbf{10.1}   &  \textbf{17.2}    &  \textbf{11.2} & \textbf{2.82} & \textbf{0.87} \\
\end{tabular}

\caption{Audio-visual speech separation results on the VoxCeleb2 dataset. We show the performance separately for seen-heard test set and unseen-unheard test set. Higher is better for all metrics.
}
\vspace{-0.05in}
\label{Table:av-speech-separation-supp}
\end{table*}

%===========================================================
\section{Ablation Study on Loss Terms}

We perform an ablation study to examine the impact
of the key components of our \textsc{VisualVoice} framework. We empirically set $\lambda_1$ and $\lambda_2$ by tuning on validation data. Note that the loss terms are not normalized for similar scales, so the absolute values of the loss weights do not directly indicate their impact on learning. Table~\ref{Table:ablation} compares the speech separation performance of several variants of our model on the VoxCeleb2 dataset. We compare our model with one variant that only uses the mask-prediction loss; one variant without using the cross-modal matching loss; one variant without using the speaker consistency loss. We can see that the mask-prediction loss provides the main supervision for learning speech \KG{separation}.  % and achieves decent results on its own.
Together with the cross-modal matching loss and speaker consistency loss, we achieve the best results both for our full model and our static face based model. It's possible that a more rigorous hyperparameter search of the loss weights can lead to better performance.   

\begin{table*}[ht]
\begin{tabular}{c?{0.5mm}ccccc?{0.5mm}ccccc}
\multirow{2}{*}{} & \multicolumn{5}{c?{0.5mm}}{Ours (static face)} & \multicolumn{5}{c}{Ours} \\ \cline{2-11} 
                  & SDR    & SIR    & SAR   & PESQ & STOI & SDR    & SIR    & SAR  & PESQ & STOI \\ \specialrule{.12em}{.1em}{.1em}
Only mask prediction loss  &   6.69     &     10.9       &  10.3    &  2.43  & 0.75  &  9.81     &     16.4       & 10.9    &  2.76  & 0.82\\ 
Without cross-modal matching loss         &  6.95   &  11.4    &  10.4  & 2.48 & 0.77  & 9.93      &   16.7 &   11.1     &   2.79  & 0.84 \\ 
Without  speaker consistency loss        &   7.10     &  11.7    &   10.4     &  2.50  & 0.79  & 10.0      &  17.0    &   11.1     &  2.81  & 0.86\\ 
All losses       &  \textbf{7.21}   &  \textbf{12.0}    &  \textbf{10.6} & \textbf{2.52} & \textbf{0.80} & \textbf{10.2}      &    \textbf{17.2}    &     \textbf{11.3}   &     \textbf{2.83}     & \textbf{0.87}   \\
\end{tabular}

\caption{Ablation study on the loss terms. Higher is better for all metrics.
}
\vspace{-0.05in}
\label{Table:ablation}
\end{table*}

%===========================================================
\section{Best/Worst Performing Pairs}

\begin{figure}[t]
    \center
    \includegraphics[scale=0.425]{images/successVSfailure.pdf}
    \caption{Qualitative examples of the best performing pairs (first row) and worst performing pairs (second row) for our static-face image based model.}
    \label{fig:successVSfailure}
    \vspace*{-0.05in}
\end{figure}

\begin{figure}[t]
    \center
    \includegraphics[scale=0.29]{images/pair_improvement.pdf}
    \caption{Qualitative examples of the pairs with the largest improvement from cross-modal face-voice embeddings.}
    \label{fig:pair_improvement}
    \vspace*{-0.05in}
\end{figure}

Fig.~\ref{fig:successVSfailure} illustrates the best and worst performing pairs for speech separation using synthetic pairs for our static face model. Pairs that perform the best tend to be very different in terms of facial attributes like gender, age, and nationality (first row). Speech separation can be hard if the two mixed identities are visually similar or the facial attributes are hard to obtain from only a static face image due to occlusion or irregular pose (second row). 

To further understand when the cross-modal face-voice embeddings help the most, we compare the per-pair performance of our model with only lip motion and our full model in Fig.~\ref{fig:pair_improvement}. The pairs with the largest improvement from the cross-modal face-voice embeddings tend to be those that either have very different facial appearances or whose lip motion cues are difficult to extract (\eg, non-frontal views).

%===========================================================
\section{Network and Implementation Details}

Our audio-visual speech separator network uses the visual cues in the face track to guide the speech separation for each speaker. The visual stream of our network consists of two parts: a lip motion analysis network and a facial attributes analysis network.

The lip motion analysis network takes $64$ mouth regions of interest (ROIs) as input. To obtain the ROIs from the face track, we use an SFD face detector~\cite{zhang2017s3fd} to detect 68 facial landmarks. Following~\cite{martinez2020lipreading}, the faces are then aligned to a mean reference face to remove differences related to rotation and scale using a similarity transformation. A $96 \times 96$ ROI is cropped once the center of the mouth is located for each frame. During training, we use random horizontal flippling, random croping of size of $88 \times 88$. During testing, the center patch is used. We use gray-scale images for the mouth ROIs as the input to the lip motion analysis network, which consists of a 3D convolutional layer with kernel $5 \times 7 \times 7$ followed by a ShuffleNet-V2 network and a temporal convolutional network. The temporal convolutional network takes the time-indexed sequence of feature vectors extracted from the ShuffleNet-V2 network, and maps it into another such sequency through the use of a 1D temporal convolution. See~\cite{martinez2020lipreading} for details. Finally, we obtain a feature map of lip motion of dimension $512 \times 64$.

The face attributes analysis network is a ResNet-18 network that takes an image of size $224 \times 224$ as input, and the feature map after the final pooling layer is downsampled to dimension of $V_f = 128$ through a fully-connected layer. We replicate the facial attributes feature along the time dimension to concatenate with the lip motion feature map and obtain a final visual feature of dimension $640 \times 64$. 

On the audio side, we use a U-Net~\cite{ronneberger2015u} style network similar to~\cite{gao2019coseparation,zhao2019som,gao2019visualsound}, but here we tailor the network to audio-visual speech separation. It consists of an encoder and a decoder network. The input to the encoder is the complex spectrogram of the mixture signal of dimension $2 \times 257 \times 256$. The input is first passed through 2 convolutional layers (kernel size = 4, stride = 2, padding = 1) that downsample the frequency and time dimension until the time dimension is equal to $N = 64$. Then we use 6 conv-blocks that each consist of two convolutional layers (kernel size = 3, stride = 1, padding = 1) followed by a frequency pooling layer. The first two convolutional layers in each conv-block preserve the spatial dimension and the frequency pooling layer after it reduces the frequency dimension by a factor of 2 while preserving the time dimension. Next, we use a $\mathtt{Tanh}$ layer to map the output feature map values to the range of [-1, 1]. Because the real and imaginary parts of the ground-truth complex mask typically lie between -5 and 5, we further use a $\mathtt{Scaling}$ operation to scale the output by 5. Finally, we obtain a bounded predicted complex mask of the same dimension as the input spectrogram for the speaker. In source separation tasks, spectrogram masks have proven better than alternatives such as direct prediction of spectrograms or raw waveforms~\cite{ephrat2018looking,gao2019coseparation}. The 1D time series audio signal varies widely with small
distortions, and perceptual information is difficult to extract
directly. STFT separates the frequencies and amplitudes,
generating a spectrogram that is more structured and can
be analyzed similarly to an image using a CNN. The mask
makes the prediction target bounded and further regularizes the learning process.

The voice attributes analysis network has the same configuration as the face attributes analysis network except the first layer of the ResNet-18 network takes the separated complex spectrogram of dimension $2 \times 256 \times 256$ as input. Similarly, the feature map after the final pooling layer is downsampled to dimension of 128 through a fully-connected layer.

%===========================================================
\section{Dataset Details}
Our experiments on audio-visual speech separation and enhancement are mainly on the VoxCeleb2 dataset due to the availability of the pre-computed face tracks and identity labels, which allow us to explicitly test for speaker-independent performance. For audio-visual enhancement experiments, we additionally mix the speech mixture with non-speech audios in AudioSet~\cite{gemmeke2017audio} (excluding the speech category from the ontology) as background noise. We mix with audios from the official training split / evaluation split during training and testing, respectively.

%AV Speech is a large dataset that contains video segments with clean speech.

We also evaluate on four standard benchmark datasets below to compare our model with a series of state-of-the-art audio-visual speech separation and enhancement methods in Sec.4.3.2 in the main paper: 1) \textbf{Mandarin~\cite{hou2018audio}} is an audio-visual dataset prepared by Hou~\etal~\cite{hou2018audio} containing video recordings of Mandarin sentences spoken by a native speaker. Each sentence is approximately 3-4 seconds and contains 10 Chinese characters with the phonemes designed to distribute equally. We use the official test set that contains 40 clean utterances, mixed with the 10 noise types (\eg, crying, music, offscreen speakers, \etc) at 5 dB, 0 dB, and -5 dB SIRs and car engine ambient noise; 2) \textbf{TCD-TIMIT~\cite{harte2015tcd}} consists of 59 volunteer speakers with around 200 videos each. The speakers are recorded saying various sentences from the TIMIT dataset. We mix every clip with another clip of a random speaker to evaluate the speech separation performance; 3) \textbf{CUAVE~\cite{patterson2002cuave}} is an audio-visual speech database consisting of videos of connected and continuous digits spoken in different situations by various speakers. The ground-truth audio for one speaker in the mixture is avaialble to evaluate the separation performance; 4) \textbf{LRS2~\cite{afouras2018deep}} is a dataset for lip reading that consists of 224 hours of videos long with pre-computed face tracks of the speakers. We follow the setting of~\cite{Afouras20audio-visual-objects} and evaluate our model using only videos that are between 2 - 5 seconds long.

%===========================================================
